# Supplementary material for: ExtraNeRF: Visibility-Aware View Extrapolation of Neural Radiance Fields with Diffusion Models
Source: arXiv:2406.06133 source file (2024-06-10)
Supplement: Supplementary file 2 [file ablation_supp.tex]

\begin{figure*}[t] 
  \centering
\includegraphics[width=\linewidth]{src/images/ablations_supp.png}
\caption{\textbf{Ablation study (Supplementary Material).}
The example in top row shows that our diffusion enhancer can introduce more detail, and the example in the bottom row shows that it can correct from color drift problem compared to using diffusion inpainter only.
}
\label{fig:ablations_supp}
\end{figure*}
